# Supplementary material for: Temporal Representation Learning for Stock Similarities and Its Applications in Investment Management
Source: arXiv:2407.13751 source file (2024-07-18)
Supplement: Supplementary file 1 [file Pair_trading_wealth_mdd_top1_2021.tex]

\useunder{\uline}{\ul}{}
\fontsize{7}{8}\selectfont{
\begin{tabular}{cccccc|ccccc}
\hline
\multirow{2}{*}{\textbf{\begin{tabular}[c]{@{}c@{}}Query\\ Stock\end{tabular}}} & \multicolumn{5}{c|}{\textbf{Wealth}}                                                         & \multicolumn{5}{c}{\textbf{Maximum Drawdown (\%)}}                                     \\
                                                                                & \textbf{SimStock} & \textbf{TS2VEC}  & \textbf{Corr1}   & \textbf{Corr2}  & \textbf{Coint}   & \textbf{SimStock} & \textbf{TS2VEC} & \textbf{Corr1} & \textbf{Corr2} & \textbf{Coint} \\ \hline
AAPL                                                                            & {\ul 1297.62}     & \textbf{1368.86} & 448.76           & -477.49         & 3273.8           & {\ul -2.25}       & \textbf{-0.46}  & -3.16          & -11.6          & -2.33          \\
CMG                                                                             & \textbf{662.32}   & -126.95          & -318.73          & -1900.87        & -864.86          & -5.68             & {\ul -4.92}     & -7.5           & -24.78         & \textbf{-4.41} \\
MSFT                                                                            & 804.26            & \textbf{1277.58} & {\ul 1036.84}    & 498.00          & -1009.7          & \textbf{-3.82}    & {\ul -5.42}     & -5.55          & -5.92          & -9.89          \\
WFC                                                                             & \textbf{790.60}   & {\ul 480.85}     & 19.30            & \textbf{790.60} & 347.59           & \textbf{-0.05}    & -5.74           & -6.82          & \textbf{-0.05} & {\ul -2.52}    \\
V                                                                               & \textbf{239.17}   & \textbf{239.17}  & \textbf{239.17}  & \textbf{239.17} & {\ul -784.11}    & \textbf{0.00}     & \textbf{0.00}   & \textbf{0.00}  & \textbf{0.00}  & -5.07          \\
XOM                                                                             & {\ul -977.06}     & {\ul -977.06}    & \textbf{-111.18} & -1182.94        & NaN              & {\ul -11.41}      & {\ul -11.41}    & \textbf{-6.64} & -14.22         & NaN            \\
PFE                                                                             & -73.56            & NaN              & {\ul 879.06}     & 90.58           & \textbf{1134.76} & {\ul -5.69}       & NaN             & \textbf{-1.88} & -8.07          & -8.2           \\
AMZN                                                                            & 680.85            & {\ul 1418.49}    & -1743.54         & -612.75         & \textbf{4101.56} & {\ul -5.68}       & \textbf{-0.01}  & -22.64         & -10.88         & -6.9           \\
BA                                                                              & \textbf{1321.94}  & {\ul 117.80}     & -921.89          & -1293.48        & -693.48          & \textbf{-3.66}    & {\ul -6.71}     & -11.96         & -15.8          & -9.2           \\
MSFT                                                                            & \textbf{559.63}   & -3543.29         & NaN              & {\ul 479.96}    & NaN              & \textbf{-1.00}    & {\ul -27.68}    & NaN            & -6.48          & NaN            \\
MA                                                                              & \textbf{196.77}   & \textbf{196.77}  & \textbf{196.77}  & \textbf{196.77} & {\ul -29.34}     & \textbf{0.00}     & \textbf{0.00}   & \textbf{0.00}  & \textbf{0.00}  & {\ul -1.94}    \\
CVS                                                                             & {\ul 1046.01}     & -523.46          & \textbf{2198.5}  & 523.24          & -111.44          & \textbf{-2.58}    & -9.36           & -10.24         & -9.96          & {\ul -8.86}    \\ \hline
\end{tabular}}
