# Supplementary material for: Temporal Representation Learning for Stock Similarities and Its Applications in Investment Management
Source: arXiv:2407.13751 source file (2024-07-18)
Supplement: Supplementary file 2 [file portfolio_MV_10.tex]

\fontsize{8}{9}\selectfont{
\begin{tabular}{rcccccccc}
\hline
\multicolumn{1}{c}{\multirow{2}{*}{Evaluation Method}} & \multicolumn{8}{c}{MinVariance - 10 Stocks}                                                \\ \cline{2-9} 
\multicolumn{1}{c}{}                                   & \multicolumn{4}{c}{S\&P500}                            & \multicolumn{4}{c}{JPX Prime 150} \\ \hline
\multicolumn{1}{r|}{Covariance Method}                 & SS     & HC     & SM     & \multicolumn{1}{c|}{GS}     & SS     & HC     & SM     & GS     \\ \hline
\multicolumn{1}{r|}{Arithmetic Return (\%)}             & 5.06   & 1.3    & 1.16   & \multicolumn{1}{c|}{1.69}   & 11.94  & 9.22   & 9.21   & 8.95   \\ \cline{1-1}
\multicolumn{1}{r|}{Geometric Return (\%)}              & 3.96   & 0.76   & 0.83   & \multicolumn{1}{c|}{1.27}   & 11.44  & 9.03   & 9.03   & 8.77   \\ \cline{1-1}
\multicolumn{1}{r|}{Cumulative Return (\%)}             & 14.23  & 3.54   & 3.44   & \multicolumn{1}{c|}{4.85}   & 39.46  & 30.12  & 29.97  & 29.21  \\ \cline{1-1}
\multicolumn{1}{r|}{Annualized SD (\%)}                 & 23.91  & 20.04  & 18.53  & \multicolumn{1}{c|}{19.04}  & 15.44  & 13.32  & 12.26  & 12.59  \\ \cline{1-1}
\multicolumn{1}{r|}{Annualized Skewness}               & 0.05   & -0.16  & -0.05  & \multicolumn{1}{c|}{-0.1}   & -0.28  & -0.15  & -0.24  & -0.26  \\ \cline{1-1}
\multicolumn{1}{r|}{Annualized Kurtosis}               & 2.54   & 2.91   & 2.72   & \multicolumn{1}{c|}{2.72}   & 2.54   & 2.78   & 2.85   & 2.76   \\ \cline{1-1}
\multicolumn{1}{r|}{Maximum Drawdown (\%)}              & -22.65 & -23.23 & -20.72 & \multicolumn{1}{c|}{-21.04} & -11.04 & -10.02 & -8.52  & -9.32  \\ \cline{1-1}
\multicolumn{1}{r|}{Monthly 95\% VaR (\%)}               & -9.39  & -8.31  & -7.72  & \multicolumn{1}{c|}{-7.99}  & -5.75  & -4.74  & -4.43  & -4.59  \\ \cline{1-1}
\multicolumn{1}{r|}{Sharpe Ratio}                      & 0.11   & -0.11  & -0.12  & \multicolumn{1}{c|}{-0.08}  & 0.94   & 0.79   & 0.86   & 0.81   \\ \cline{1-1}
\multicolumn{1}{r|}{Annualized Turnover}               & 1.14   & 4.65   & 3.82   & \multicolumn{1}{c|}{4.11}   & 1.25   & 4.65   & 3.28   & 3.98   \\ \cline{1-1}
\multicolumn{1}{r|}{Portfolio wealth}                  & 114229 & 104854 & 103438 & \multicolumn{1}{c|}{103537} & 139459 & 129207 & 129970 & 130123 \\ \hline
\end{tabular}}
