# Supplementary material for: Temporal Representation Learning for Stock Similarities and Its Applications in Investment Management
Source: arXiv:2407.13751 source file (2024-07-18)
Supplement: Supplementary file 3 [file portfolio_MV_50.tex]

\fontsize{8}{9}\selectfont{
\begin{tabular}{rcccccccc}
\hline
\multicolumn{1}{c}{\multirow{2}{*}{Evaluation Method}} & \multicolumn{8}{c}{MinVariance - 50 Stocks}                                                \\ \cline{2-9} 
\multicolumn{1}{c}{}                                   & \multicolumn{4}{c}{S\&P500}                            & \multicolumn{4}{c}{JPX Prime 150} \\ \hline
\multicolumn{1}{r|}{Covariance Method}                 & SS     & HC     & SM     & \multicolumn{1}{c|}{GS}     & SS     & HC     & SM     & GS     \\ \hline
\multicolumn{1}{r|}{Arithmetic Return (\%)}             & 2.53   & 0.74   & -0.47  & \multicolumn{1}{c|}{0.17}   & 12.61  & 13.72  & 12.29  & 13.42  \\ \cline{1-1}
\multicolumn{1}{r|}{Geometric Return (\%)}              & 1.72   & 0.34   & -0.73  & \multicolumn{1}{c|}{-0.13}  & 12.21  & 13.40  & 12.14  & 13.18  \\ \cline{1-1}
\multicolumn{1}{r|}{Cumulative Return (\%)}             & 6.33   & 1.88   & -1.8   & \multicolumn{1}{c|}{0.06}   & 41.79  & 46.23  & 41.17  & 45.23  \\ \cline{1-1}
\multicolumn{1}{r|}{Annualized SD (\%)}                 & 23.69  & 19.34  & 16.14  & \multicolumn{1}{c|}{17.51}  & 14.14  & 12.22  & 9.47   & 10.45  \\ \cline{1-1}
\multicolumn{1}{r|}{Annualized Skewness}               & 0.04   & -0.25  & 0.12   & \multicolumn{1}{c|}{0}      & -0.36  & 0.11   & 0.00   & -0.08  \\ \cline{1-1}
\multicolumn{1}{r|}{Annualized Kurtosis}               & 2.48   & 3.24   & 3      & \multicolumn{1}{c|}{2.93}   & 2.68   & 2.74   & 2.86   & 2.73   \\ \cline{1-1}
\multicolumn{1}{r|}{Maximum Drawdown (\%)}              & -24.1  & -22.34 & -19.18 & \multicolumn{1}{c|}{-19.82} & -9.15  & -8.14  & -4.59  & -5.90  \\ \cline{1-1}
\multicolumn{1}{r|}{Monthly 95\% VaR (\%)}               & -9.44  & -8.12  & -7.05  & \multicolumn{1}{c|}{-7.39}  & -5.34  & -3.57  & -2.90  & -3.11  \\ \cline{1-1}
\multicolumn{1}{r|}{Sharpe Ratio}                      & -0.03  & -0.15  & -0.28  & \multicolumn{1}{c|}{-0.21}  & 1.13   & 1.45   & 1.63   & 1.64   \\ \cline{1-1}
\multicolumn{1}{r|}{Annualized Turnover}               & 1.21   & 7.5    & 5.68   & \multicolumn{1}{c|}{6.48}   & 1.23   & 8.39   & 4.49   & 6.44   \\ \cline{1-1}
\multicolumn{1}{r|}{Portfolio wealth}                  & 106331 & 100059 & 98195  & \multicolumn{1}{c|}{101878} & 141792 & 145230 & 141172 & 146234 \\ \hline
\end{tabular}}
