# Supplementary material for: Temporal Representation Learning for Stock Similarities and Its Applications in Investment Management
Source: arXiv:2407.13751 source file (2024-07-18)
Supplement: Supplementary file 4 [file portfolio_stock_10_SNP.tex]

\fontsize{8}{9}\selectfont{
\begin{tabular}{r|cccc|cccc|cccc|cccc}
\hline
S\&P500 | 10 Stocks    & \multicolumn{4}{c|}{Target Volatility (24\%)} & \multicolumn{4}{c|}{Target Volatility (27\%)} & \multicolumn{4}{c|}{Target Volatility (30\%)} & \multicolumn{4}{c}{Target Volatility (33\%)} \\ \hline
Covariance Method     & SS        & HC        & SM        & GS       & SS        & HC        & SM        & GS       & SS        & HC        & SM        & GS       & SS        & HC        & SM       & GS       \\ \hline
Arithmetic Return (\%) & 7.94      & 6.85      & 6.84      & 6.97     & 8.38      & 7.35      & 7.27      & 7.27     & 8.56      & 7.71      & 7.8       & 7.71     & 8.84      & 8.12      & 8.27     & 8.13     \\ \cline{1-1}
Geometric Return (\%)  & 6.78      & 6.05      & 6.08      & 6.11     & 7.1       & 6.41      & 6.34      & 6.25     & 7.18      & 6.61      & 6.68      & 6.51     & 7.31      & 6.85      & 6.98     & 6.77     \\ \cline{1-1}
Cumulative Return (\%) & 24.63     & 22.11     & 22.11     & 22.32    & 26.26     & 23.73     & 23.49     & 23.19    & 26.79     & 24.73     & 25.05     & 24.39    & 27.52     & 25.71     & 26.3     & 25.53    \\ \cline{1-1}
Annualized SD (\%)     & 27.22     & 24.68     & 24.57     & 25.06    & 28.18     & 26.06     & 26.11     & 26.49    & 29.11     & 27.31     & 27.47     & 27.79    & 29.94     & 28.44     & 28.67    & 28.92    \\ \cline{1-1}
Annualized Skewness   & -0.06     & -0.06     & -0.03     & -0.03    & -0.08     & -0.07     & -0.06     & -0.06    & -0.09     & -0.08     & -0.07     & -0.08    & -0.1      & -0.08     & -0.08    & -0.08    \\ \cline{1-1}
Annualized Kurtosis   & 3.04      & 3.06      & 3.04      & 3.04     & 3.09      & 3.08      & 3.07      & 3.07     & 3.12      & 3.12      & 3.11      & 3.11     & 3.15      & 3.15      & 3.15     & 3.15     \\ \cline{1-1}
Maximum Drawdown (\%)  & -26.07    & -24.22    & -24.04    & -24.4    & -27.13    & -25.28    & -25.23    & -25.73   & -27.93    & -26.52    & -26.41    & -26.93   & -28.59    & -27.49    & -27.46   & -27.85   \\ \cline{1-1}
Monthly 95\% VaR (\%)   & -10.24    & -9.43     & -9.39     & -9.57    & -10.62    & -9.92     & -9.93     & -10.06   & -11       & -10.3     & -10.36    & -10.49   & -11.28    & -10.7     & -10.76   & -10.85   \\ \cline{1-1}
Sharpe Ratio          & 0.24      & 0.22      & 0.23      & 0.23     & 0.25      & 0.23      & 0.23      & 0.22     & 0.25      & 0.23      & 0.23      & 0.22     & 0.24      & 0.23      & 0.24     & 0.23     \\ \cline{1-1}
Annualized Turnover   & 7.15      & 6.81      & 6.88      & 6.94     & 7.31      & 7         & 7.09      & 7.15     & 7.22      & 7.15      & 7.21      & 7.25     & 7.23      & 7.21      & 7.24     & 7.26     \\ \cline{1-1}
Portfolio wealth      & 124628    & 122319    & 122110    & 122111   & 126259    & 123189    & 123492    & 123734   & 126786    & 124393    & 125048    & 124726   & 127523    & 125530    & 126303   & 125707   \\ \hline
\end{tabular}}
