# Supplementary material for: Temporal Representation Learning for Stock Similarities and Its Applications in Investment Management
Source: arXiv:2407.13751 source file (2024-07-18)
Supplement: Supplementary file 5 [file portfolio_stock_10_TSE.tex]

\fontsize{8}{9}\selectfont{
\begin{tabular}{r|cccc|cccc|cccc|cccc}
\hline
JPM Prime 150 | 10 Stocks & \multicolumn{4}{c|}{Target Volatility (24\%)}                                                                       & \multicolumn{4}{c|}{Target Volatility (27\%)}                                                                       & \multicolumn{4}{c|}{Target Volatility (30\%)}                                                                       & \multicolumn{4}{c}{Target Volatility (33\%)}                                                                       \\ \hline
Covariance Method         & SS                         & HC                         & SM                         & GS                          & SS                         & HC                         & SM                         & GS                          & SS                         & HC                         & SM                         & GS                          & SS                         & HC                         & SM                         & GS                         \\ \hline
Arithmetic Return (\%)     & 15.63                      & 14.41                      & 14.51                      & 14.4                        & 16.19                      & 15.43                      & 15.67                      & 15.55                       & 16.59                      & 16.43                      & 16.74                      & 16.7                        & 17.64                      & 17.4                       & 17.42                      & 17.55                      \\ \cline{1-1}
Geometric Return (\%)      & 13.94                      & 13.17                      & 13.1                       & 13.06                       & 14.28                      & 13.88                      & 13.92                      & 13.86                       & 14.55                      & 14.6                       & 14.68                      & 14.71                       & 15.34                      & 15.32                      & 15.17                      & 15.32                      \\ \cline{1-1}
Cumulative Return (\%)     & 53                         & 49.12                      & 48.85                      & 48.69                       & 55.09                      & 53.04                      & 53.44                      & 53.24                       & 56.99                      & 56.99                      & 57.98                      & 58.02                       & 61.27                      & 61.1                       & 61.09                      & 61.66                      \\ \cline{1-1}
Annualized SD (\%)         & 25.93                      & 25.05                      & 24.8                       & 25.09                       & 27.34                      & 27.01                      & 27.09                      & 27.21                       & 28.65                      & 28.89                      & 29.18                      & 29.27                       & 29.97                      & 30.61                      & 30.89                      & 30.95                      \\ \cline{1-1}
Annualized Skewness       & 0.18                       & 0.25                       & 0.24                       & 0.21                        & 0.21                       & 0.28                       & 0.3                        & 0.27                        & 0.24                       & 0.32                       & 0.33                       & 0.3                         & 0.24                       & 0.32                       & 0.34                       & 0.32                       \\ \cline{1-1}
Annualized Kurtosis       & 3.55                       & 3.3                        & 3.33                       & 3.3                         & 3.64                       & 3.38                       & 3.43                       & 3.38                        & 3.73                       & 3.46                       & 3.52                       & 3.45                        & 3.69                       & 3.51                       & 3.58                       & 3.53                       \\ \cline{1-1}
Maximum Drawdown (\%)      & -21.1                      & -20.52                     & -20.56                     & -20.88                      & -22.37                     & -22                        & -22.29                     & -22.6                       & -23.38                     & -23.38                     & -23.89                     & -24.09                      & -24.44                     & -24.78                     & -25.24                     & -25.36                     \\ \cline{1-1}
Monthly 95\% VaR (\%)       & -8.83                      & -8.76                      & -8.61                      & -8.81                       & -9.35                      & -9.41                      & -9.29                      & -9.48                       & -9.78                      & -9.97                      & -10                        & -10.1                       & -10.18                     & -10.46                     & -10.5                      & -10.57                     \\ \cline{1-1}
Sharpe Ratio              & 0.68                       & 0.65                       & 0.66                       & 0.65                        & 0.66                       & 0.64                       & 0.64                       & 0.64                        & 0.64                       & 0.63                       & 0.63                       & 0.63                        & 0.64                       & 0.63                       & 0.62                       & 0.62                       \\ \cline{1-1}
Annualized Turnover       & 7.28                       & 7.56                       & 7.47                       & 7.53                        & 7.45                       & 7.67                       & 7.59                       & 7.63                        & 7.57                       & 7.71                       & 7.64                       & 7.65                        & 7.75                       & 7.68                       & 7.63                       & 7.61                       \\ \cline{1-1}
Portfolio wealth          & \multicolumn{1}{r}{152998} & \multicolumn{1}{r}{148687} & \multicolumn{1}{r}{148846} & \multicolumn{1}{r|}{149122} & \multicolumn{1}{r}{155091} & \multicolumn{1}{r}{153245} & \multicolumn{1}{r}{153443} & \multicolumn{1}{r|}{153042} & \multicolumn{1}{r}{156989} & \multicolumn{1}{r}{158017} & \multicolumn{1}{r}{157977} & \multicolumn{1}{r|}{156985} & \multicolumn{1}{r}{161269} & \multicolumn{1}{r}{161661} & \multicolumn{1}{r}{161087} & \multicolumn{1}{r}{161102} \\ \hline
\end{tabular}}
