# Supplementary material for: Temporal Representation Learning for Stock Similarities and Its Applications in Investment Management
Source: arXiv:2407.13751 source file (2024-07-18)
Supplement: Supplementary file 6 [file portfolio_stock_50_SNP.tex]

\fontsize{8}{9}\selectfont{
\begin{tabular}{r|cccc|cccc|cccc|cccc}
\hline
S\&P500 | 50 Stocks    & \multicolumn{4}{c|}{Target Volatility (24\%)} & \multicolumn{4}{c|}{Target Volatility (27\%)} & \multicolumn{4}{c|}{Target Volatility (30\%)} & \multicolumn{4}{c}{Target Volatility (33\%)} \\ \hline
Covariance Method     & SS        & HC        & SM        & GS       & SS        & HC        & SM        & GS       & SS        & HC        & SM        & GS       & SS        & HC        & SM       & GS       \\ \hline
Arithmetic Return (\%) & 10.41     & 10.27     & 9.82      & 10.54    & 11.86     & 11.15     & 11.38     & 11.59    & 12.82     & 12.1      & 12.7      & 12.67    & 13.87     & 13.03     & 13.78    & 13.57    \\ \cline{1-1}
Geometric Return (\%)  & 9.59      & 9.5       & 9.19      & 9.84     & 10.92     & 10.24     & 10.57     & 10.71    & 11.74     & 11.01     & 11.66     & 11.56    & 12.57     & 11.73     & 12.47    & 12.27    \\ \cline{1-1}
Cumulative Return (\%) & 34.15     & 33.49     & 32.06     & 34.49    & 39.14     & 36.27     & 37.5      & 38.06    & 42.3      & 39.41     & 41.93     & 41.71    & 45.6      & 42.45     & 45.44    & 44.76    \\ \cline{1-1}
Annualized SD (\%)     & 29        & 27.93     & 27.2      & 27.53    & 30.6      & 29.67     & 29.42     & 29.58    & 32.34     & 31.38     & 31.54     & 31.64    & 33.92     & 33.07     & 33.47    & 33.52    \\ \cline{1-1}
Annualized Skewness   & -0.17     & -0.22     & -0.19     & -0.18    & -0.2      & -0.25     & -0.24     & -0.23    & -0.23     & -0.27     & -0.27     & -0.26    & -0.26     & -0.29     & -0.31    & -0.29    \\ \cline{1-1}
Annualized Kurtosis   & 3.12      & 3.28      & 3.32      & 3.19     & 3.18      & 3.35      & 3.36      & 3.27     & 3.24      & 3.37      & 3.4       & 3.31     & 3.24      & 3.36      & 3.38     & 3.3      \\ \cline{1-1}
Maximum Drawdown (\%)  & -25.4     & -24.36    & -23.35    & -23.44   & -25.79    & -25.44    & -24.66    & -24.97   & -26.33    & -26.6     & -25.94    & -26.53   & -27.29    & -27.68    & -27.34   & -27.85   \\ \cline{1-1}
Monthly 95\% VaR (\%)   & -10.96    & -10.36    & -10.15    & -10.18   & -11.28    & -10.79    & -10.78    & -10.82   & -11.64    & -11.2     & -11.3     & -11.29   & -12.06    & -11.68    & -11.8    & -11.79   \\ \cline{1-1}
Sharpe Ratio          & 0.39      & 0.41      & 0.39      & 0.43     & 0.44      & 0.42      & 0.44      & 0.45     & 0.46      & 0.43      & 0.46      & 0.46     & 0.48      & 0.44      & 0.47     & 0.47     \\ \cline{1-1}
Annualized Turnover   & 8.94      & 8.57      & 8.69      & 8.5      & 8.9       & 8.63      & 8.74      & 8.57     & 8.84      & 8.66      & 8.67      & 8.6      & 8.7       & 8.63      & 8.55     & 8.54     \\ \cline{1-1}
Portfolio wealth      & 134152    & 134488    & 132064    & 133490   & 139140    & 138057    & 137496    & 136267   & 142298    & 141706    & 141925    & 139414   & 145597    & 144761    & 145442   & 142451   \\ \hline
\end{tabular}}
