# Supplementary material for: Temporal Representation Learning for Stock Similarities and Its Applications in Investment Management
Source: arXiv:2407.13751 source file (2024-07-18)
Supplement: Supplementary file 7 [file portfolio_stock_50_TSE.tex]

\fontsize{8}{9}\selectfont{
\begin{tabular}{r|cccc|cccc|cccc|cccc}
\hline
JPM Prime 150 | 50 Stocks & \multicolumn{4}{c|}{Target Volatility (24\%)}                                                                       & \multicolumn{4}{c|}{Target Volatility (27\%)}                                                                       & \multicolumn{4}{c|}{Target Volatility (30\%)}                                                                       & \multicolumn{4}{c}{Target Volatility (33\%)}                                                                       \\ \hline
Covariance Method         & SS                         & HC                         & SM                         & GS                          & SS                         & HC                         & SM                         & GS                          & SS                         & HC                         & SM                         & GS                          & SS                         & HC                         & SM                         & GS                         \\ \hline
Arithmetic Return (\%)     & 20.3                       & 19.7                       & 18.6                       & 17.55                       & 21.3                       & 20.03                      & 19.79                      & 18.99                       & 22.74                      & 20.34                      & 21.2                       & 20.22                       & 23.49                      & 20.93                      & 21.93                      & 21.25                      \\ \cline{1-1}
Geometric Return (\%)      & 18.9                       & 18.52                      & 17.31                      & 16.51                       & 19.89                      & 18.79                      & 18.38                      & 17.8                        & 21.27                      & 19.04                      & 19.68                      & 18.96                       & 21.98                      & 19.52                      & 20.34                      & 19.86                      \\ \cline{1-1}
Cumulative Return (\%)     & 70.97                      & 69.2                       & 63.79                      & 59.9                        & 75.61                      & 70.44                      & 68.66                      & 65.51                       & 82.1                       & 71.7                       & 74.76                      & 70.89                       & 85.94                      & 74.21                      & 78.27                      & 75.42                      \\ \cline{1-1}
Annualized SD (\%)         & 28.13                      & 27.37                      & 26.14                      & 26.54                       & 29.89                      & 28.77                      & 28.08                      & 28.34                       & 31.52                      & 30.25                      & 29.98                      & 30.02                       & 33.01                      & 31.65                      & 31.42                      & 31.43                      \\ \cline{1-1}
Annualized Skewness       & -0.03                      & 0                          & -0.01                      & -0.01                       & 0.02                       & -0.03                      & 0.02                       & 0.01                        & 0.03                       & -0.03                      & 0.02                       & -0.01                       & 0.03                       & -0.06                      & -0.02                      & -0.07                      \\ \cline{1-1}
Annualized Kurtosis       & 2.89                       & 2.86                       & 2.83                       & 2.79                        & 2.88                       & 2.88                       & 2.9                        & 2.87                        & 2.89                       & 2.88                       & 2.93                       & 2.88                        & 2.9                        & 2.91                       & 2.91                       & 2.91                       \\ \cline{1-1}
Maximum Drawdown (\%)      & -21.47                     & -20.57                     & -20.47                     & -20.64                      & -22.41                     & -21.99                     & -21.58                     & -21.61                      & -22.99                     & -23.12                     & -22.54                     & -22.45                      & -23.79                     & -24.39                     & -23.67                     & -23.67                     \\ \cline{1-1}
Monthly 95\% VaR (\%)       & -9.73                      & -9.68                      & -8.9                       & -9.27                       & -10.25                     & -10.23                     & -9.55                      & -9.87                       & -10.74                     & -10.8                      & -10.22                     & -10.51                      & -11.22                     & -11.35                     & -10.83                     & -11.18                     \\ \cline{1-1}
Sharpe Ratio              & 0.93                       & 0.93                       & 0.91                       & 0.85                        & 0.93                       & 0.9                        & 0.91                       & 0.86                        & 0.96                       & 0.87                       & 0.92                       & 0.88                        & 0.95                       & 0.85                       & 0.91                       & 0.88                       \\ \cline{1-1}
Annualized Turnover       & 8.99                       & 8.77                       & 8.98                       & 8.96                        & 9                          & 8.91                       & 9.08                       & 8.99                        & 8.91                       & 9.01                       & 9                          & 8.93                        & 8.86                       & 8.98                       & 8.97                       & 8.9                        \\ \cline{1-1}
Portfolio wealth          & \multicolumn{1}{r}{170971} & \multicolumn{1}{r}{159904} & \multicolumn{1}{r}{163786} & \multicolumn{1}{r|}{169196} & \multicolumn{1}{r}{175607} & \multicolumn{1}{r}{165507} & \multicolumn{1}{r}{168658} & \multicolumn{1}{r|}{170442} & \multicolumn{1}{r}{182095} & \multicolumn{1}{r}{170891} & \multicolumn{1}{r}{174760} & \multicolumn{1}{r|}{171696} & \multicolumn{1}{r}{185940} & \multicolumn{1}{r}{175416} & \multicolumn{1}{r}{178270} & \multicolumn{1}{r}{174212} \\ \hline
\end{tabular}}
